# Supplementary material for: MNL-Bandit: A Dynamic Learning Approach to Assortment Selection
Source: arXiv:1706.03880 source file (2018-06-29)
Supplement: Supplementary file 1 [file lower_bound_appendix.tex]

\begin{lemma}\label{right_feedback}
For any assortment $S_\ell$ suggested by \amnl, for each $i \in S_\ell$, let $\mathcal{P}_{S_\ell}(i)$ denote the probability that \amab gives the feedback that product $i$ is purchased. And, let $\mathcal{P}_{S_\ell}(0)$ denote the probability that \amab gives the feedback that no product is purchased. 
%We have the following result. 
Then, for each $i \in S_\ell \cup \{0\},$
$$\ep{P}_{S_\ell}\left( i \right) = \frac{v_i}{v_0 + \sum_{j \in S_\ell}v_j}.$$
\end{lemma}
\begin{proof}
Let $M$ denote the number of times no arm is pulled or arm ${\lceil}{\frac{i}{K}}{\rceil}$ is pulled for some $i \in S_\ell$ by $A_{MAB}$ before giving the feedback to $bandit$-MNL algorithm that a particular product has been purchased. We have 
$$ \mathcal{P}(M=m \; \cap\; \text{arm ${\lceil}{\frac{i}{K}}{\rceil}$ is pulled and observed reward is 1}) = \frac{v_i}{2K}\left( \frac{1}{2K}\sum_{i \in S_\ell} (1-v_i) \right)^{m-1}.$$
%Similarly, we have $$ \mathcal{P}(M=m \; \cap\; \text{no arm is pulled}) = \frac{1}{2}\left( \frac{1}{2K}\sum_{i \in S_\ell} (1-v_i) \right)^{m-1}.$$
Therefore we have, 
\begin{equation*}
\begin{aligned}
\mathcal{P}_{S_\ell}(i) &= \sum_{m=1}^{\infty} \mathcal{P}(M=m \; \cap\; \text{arm ${\lceil}{\frac{i}{K}}{\rceil}$ is pulled and observed reward is 1})= \displaystyle \frac{v_i}{K+\sum_{q \in S_\ell} v_q}.
\end{aligned}
\end{equation*}
\end{proof}
Let $L$ be the total number of calls to \amnl in \amab. Intuitvely, after any call  to \amnl (``{\bf Call} \amnl" in  Algorithm \ref{mab_algo}), many iterations of the following loop may be executed; in roughly $1/2$ of those iterations, an arm is pulled and $t$ is advanced (with probability $1/2$, the loop is exited without advancing $t$). Therefore, $T$ should be at least a constant fraction of $L$. Following lemma makes this intuition precise.

\begin{lemma}\label{lemmaTL}
Let $L$ be the total number of calls to \amnl when \amab is executed for $T$ time steps. Then,
$$E(L) \leq  3T.$$
\end{lemma}
\begin{proof}
Let $\eta_\ell$ be the random variable that denote the duration, assortment $S_\ell$ has been considered by $\ep{A}_{MAB}$, i.e. $\eta_\ell = 0$, if we no arm is pulled when $\ep{A}_{MNL}$ suggested assortment $S_\ell$ and $\eta_\ell \geq 1$, otherwise. We have 
$$\sum_{\ell=1}^{L-1} \eta_\ell \leq T.$$ Therefore, we have $E\left(\sum_{\ell=1}^{L-1} \eta_\ell \right) \leq T$. Note that $E(\eta_\ell) \geq \frac{1}{2}$. Hence, we have 
$E(L) \leq 2T+1 \leq 3T.$
\end{proof}

Next, we use the properties of this construction to relate regret of \amab in $T$ time steps to regret of \amnl in $L$ steps.

%\begin{lemma}\label{lemma7}
%With high probability, the time scale of the $\ep{A}_{MAB}$ and the time scale of $\ep{A}_{MNL}$ are similar in scale, i.e. 
%$$\ep{P}\left( T \leq 3L\right) \geq \Omega(1-\frac{1}{T}).$$
%\end{lemma}
%Both lemmas \ref{lemma6} and \ref{lemma7} establish that the time scales are similar in scale allowing us to compare regret for different algorithms. 

%\paragraph{}
%Let $M$ denote the number of times no arm is pulled or arm ${\lceil}{\frac{i}{K}}{\rceil}$ is pulled for some $i \in S_\ell$ by $A_{MAB}$ before giving the feedback to $bandit$-MNL algorithm that a particular product has been purchased. We have 
%$$ \mathcal{P}(M=m \; \cap\; \text{arm ${\lceil}{\frac{i}{K}}{\rceil}$ is pulled and observed reward is 1}) = \frac{v_i}{2K}\left( \frac{1}{2K}\sum_{i \in S_\ell} (1-v_i) \right)^{m-1}.$$
%Similarly, we have $$ \mathcal{P}(M=m \; \cap\; \text{no arm is pulled}) = \frac{1}{2}\left( \frac{1}{2K}\sum_{i \in S_\ell} (1-v_i) \right)^{m-1}.$$
%Therefore we have, 
%\begin{equation*}
%\begin{aligned}
%\mathcal{P}_{S_\ell}(i) &= \sum_{m=1}^{\infty} \mathcal{P}(M=m \; \cap\; \text{arm ${\lceil}{\frac{i}{K}}{\rceil}$ is pulled and observed reward is 1})\\
%&= \displaystyle \frac{v_i}{K+\sum_{q \in S_\ell} v_q},
%\end{aligned}
%\end{equation*}
%and
% 
%\begin{equation*}
%\begin{aligned}
%\mathcal{P}_{S_\ell}(0) &= \sum_{m=1}^{\infty} \mathcal{P}(M=m \; \cap\; \text{no arm is pulled})\\
%&= \displaystyle \frac{K}{K+\sum_{q \in S_\ell} v_q}.
%\end{aligned}
%\end{equation*}
\subsection{Relating regret of \amnl and \amab to prove Theorem \ref{lower_bound}} \label{relate_mnl_mab}
Let $S^*$ be the optimal assortment for $I_{MNL}$. For any instantiation of $I_{MNL}$, it is easy to see that the optimal assortment contains $K$ items, all with parameter $\alpha+\epsilon$, i.e., it contains all $i$ such that $\lceil \frac{i}{K}\rceil=j$. Therefore, $V(S^*)= K(\alpha+\epsilon) = K\mu_j$. The following lemmas relate regret of \amnl to regret of \amab by bounding both in terms of $(\sum_{\ell} V(S^*)-V(S_\ell))$.  
\begin{lemma}
Total expected regret of \amab on instance $I_{MAB}$ in $T$ time steps is upper bounded as
\begin{equation}\label{eq:MNL_MAB} Reg(\text{\amab}, T) \le \frac{1}{(1+\alpha)} E\left(\sum_{\ell=1}^L \frac{1}{K} (V(S^*) - V(S_\ell))\right),\end{equation} where the expectation in equation \eqref{eq:MNL_MAB} is over the random variables $L$ and $S_\ell$.
\end{lemma}
\begin{proof}
Fix $L$, let us label the loop following the $\ell$th call to \amnl in Algorithm \ref{mab_algo} as $\ell$th loop. 
Then, we show that the total expected regret of \amab over the arm pulls in loop $\ell$ is   
$$ \frac{V(S^*) - V(S_\ell)}{(K+ V(S_\ell))}$$
The lemma statement will then follow from substituting $V(S_\ell) \ge K\alpha$ and summing over $\ell=1,\ldots, L$ and taking expectation over the random variables. 

To see above, note that the probability of exiting the loop is \mbox{$p =E[\frac{1}{2}+\frac{1}{2}\mu_{{\cal A}_t}]$} $= \frac{1}{2}+\frac{1}{2K} V(S_\ell)$. In every step of the loop until exited, an arm is pulled with probability $1/2$. The optimal strategy would pull the best arm so that the total expected optimal reward in the loop is \mbox{$\sum_{r=1}^\infty (1-p)^{r-1} \frac{1}{2} \mu_j = \frac{\mu_j}{2p} = \frac{1}{2Kp}V(S^*)$}. Algorithm \amab pulls a random arm from $S_{\ell}$, so total expected algorithm's reward in the loop is $\sum_{r=1}^\infty (1-p)^{r-1} \frac{1}{2K} V(S_\ell) = \frac{1}{2Kp} V(S_\ell)$. Subtracting the algorithm's reward from optimal reward, and substituting $p$, we obtain the above expression for expected regret over the arm pulls in a \mbox{loop.}
\end{proof}

\begin{lemma}
Total expected regret of \amnl on instance $I_{MNL}$ in $L$ time steps is lower bounded as
$$ Reg(\text{\amnl}, L) \ge \frac{1}{(1+\alpha)} \sum_{\ell=1}^L \frac{1}{K} (V(S^*) - V(S_\ell)) - \frac{\epsilon v^* L}{(1+\alpha)^2}$$
\end{lemma}
\begin{proof}
\setlength{\belowdisplayskip}{0pt} \setlength{\belowdisplayshortskip}{0pt}
\setlength{\abovedisplayskip}{0pt} \setlength{\abovedisplayshortskip}{0pt}
\begin{eqnarray*} 
 Reg(\text{\amnl}, L) & = & \sum_{\ell=1}^L R(S^*) - R(S_\ell) \\
& = & \sum_{\ell=1}^L \frac{V(S^*)}{v_0+V(S^*)} - \frac{V(S_\ell)}{v_0+V(S_\ell)}\\
& \ge & \frac{1}{K(1+\alpha)} \sum_{\ell=1}^L \left(\frac{V(S^*)}{1+\frac{\epsilon}{1+\alpha}} - V(S_\ell)\right)\\
& \ge & \frac{1}{(1+\alpha)} \sum_{\ell=1}^L \frac{1}{K} (V(S^*) - V(S_\ell)) - \frac{\epsilon v^* L}{(1+\alpha)^2} 
\end{eqnarray*} 
\end{proof}
\proofof{ Theorem \ref{lower_bound}.}
Now we are ready to prove Theorem \ref{lower_bound}. From the previous two lemmas, we have 
\begin{equation}\label{eq:MAB_MNL} Reg(\text{\amab}, T) \le E\left(Reg(\text{\amnl}, L) +  \frac{\epsilon v^* L}{(1+\alpha)^2}\right),\end{equation} where the expectation in equation \eqref{eq:MAB_MNL} is over the random variables $L$.
Now for contradiction suppose that the regret of the \text{\amnl}, $ Reg(\text{\amnl}, L) \le c\sqrt{\frac{\hat{N}L}{K}}$ for a constant $c$ to be prescribed in the following. Then, from above and Jensen's inequality, we have, 
\begin{eqnarray*}
Reg(\text{\amab}, T) & \le &  c\sqrt{\frac{\hat{N}E(L)}{K}} +  \frac{\epsilon v^* E(L)}{(1+\alpha)^2}
\end{eqnarray*}
From lemma \ref{lemmaTL}, we have that $E(L) \leq 3T$. Therefore, we have, $c\sqrt{\frac{\hat{N}E(L)}{K}} = c\sqrt{NE(L)} \le  c\sqrt{3NT} = c\epsilon T \sqrt{\frac{3}{\alpha}} < \frac{\epsilon T}{12}$ on setting $c< \frac{1}{12}\sqrt{\frac{\alpha}{3}} $. Also, using $v^*=\alpha+\epsilon \le 2\alpha$, and $L\le 3T$, and setting $\alpha$ to be a small enough constant, we can get that the second term above is also strictly less than $\frac{\epsilon T}{12}$. Combining these observations, we have \vspace{-0.3cm}
$$ \textstyle Reg(\text{\amab}, T)  <  \frac{\epsilon T}{12} + \frac{\epsilon T}{12} = \frac{\epsilon T}{6},  \vspace{-0.3cm}	$$
thus arriving at a contradiction. This proves that $Reg(\text{\amnl}, L) > c\sqrt{\frac{\hat{N}L}{K}}$ for a constant \mbox{$c$. }
